# Supplementary material for: Quantitative comparison of the magnetic proximity effect in Pt detected by XRMR and XMCD
Source: arXiv:2010.02195 source file (2021-01-07)
Supplement: Supplementary file 1 [file Comparison_XRMR_XMCD_Supplemental_Material.pdf]

# - Supplemental Material -
# Quantitative comparison of the magnetic proximity effect in Pt detected by XRMR and XMCD


Dominik Graulich,[1, a)] Jan Krieft,[1] Anastasiia Moskaltsova,[1] Johannes Demir,[1] Tobias Peters,[1] Tobias Pohlmann,[2, 3] Florian Bertram,[3] Joachim Wollschläger,[2] Jose R. L. Mardegan,[3] Sonia Francoual,[3] and Timo Kuschel[1]

[1)] *Center for Spinelectronic Materials and Devices, Department of Physics, Bielefeld University, Universitätsstraße 25, 33615 Bielefeld, Germany*

[2)] *Center of Physics and Chemistry of New Materials, Department of Physics, Osnabrück University, Barbarastraße 7, 49076 Osnabrück, Germany*

[3)] *Deutsches Elektronen-Synchrotron DESY, Notkestraße 85, 22607 Hamburg, Germany*



(Dated: 7 December 2020)


## Experimental Details

The XRMR and XMCD measurements around the Pt $L_2$ and $L_3$ absorption edges were carried out at room temperature at the resonant scattering and diffraction beamline P09 of the third-generation synchrotron PETRA III at DESY (Hamburg, Germany)[1]. A four-coil electromagnet constructed at Bielefeld University was used to apply a magnetic field of $\pm 150\,\mathrm{mT}$ in the scattering plane and parallel to the sample surface. It was mounted on the six-circle diffractometer in the first experimental hutch of P09 (P09-EH1). The generation of circularly polarized x-rays was done using a single 850 $\mu$m thick diamond plate at quarter wave plate condition. A degree of circular polarization of 99±1% was verified by an Au(111) analyzer crystal. The XMCD measurements were carried out in a grazing angle geometry in order to maximize the sample scattering volume with an energy dispersive silicon drift fluorescence detector to isolate the Pt fluorescence from other signals. The samples were illuminated at an angle of about $\theta = 2°$. In addition, the XRMR measurements collected in a $2\theta$ range of 0.16° to 6.16° were performed using an avalanche photodiode mounted on the $2\theta$-arm of the diffractometer.

The samples were both measured along the magnetic hard axis of the FM. For Pt(3.4 nm)/Fe(10.2 nm)//MgO(001), the sample was 5x10 $\mathrm{mm}^2$ and positioned with the long side parallel to the beam direction, hence along the Fe[110]//MgO[100] direction. For Pt(3.8 nm)/$Co_{33}Fe_{67}$(10.0 nm)//MgO(001) the sample had a dimension of 10x10 $\mathrm{mm}^2$ and was placed with the diagonal along the beam direction, hence $Co_{33}Fe_{67}$[100]//MgO[110]. While both samples were measured along the magnetic hard axis of the FM, saturation of the FM in similar samples was shown in Ref.[2] to be achieved below the external magnetic field of 150 mT used in the present study.

## Theoretical Background

In general, XRMR can either be measured with fixed polarization of the incident x-rays and a variation of the external magnetic field at every scattering vector, thus switching the magnetization of the sample. Or it can be measured with a fixed external magnetic field and flipping the x-ray helicity at every scattering vector. In both cases, the magnetic circular dichroism results in a change of the refractive index $n = 1 - \delta + i\beta$ within the spin-polarized material with dispersion $\delta$ and absorption $\beta$. These magnetooptic changes $\pm\Delta\delta$ and $\pm\Delta\beta$ are different for different magnetization directions or x-ray polarizations ($\pm$). The asymmetry caused by the slightly different XRR curves for varying magnetization directions or x-ray helicities allows for the evaluation of the magnetooptic depth profiles of $\Delta\delta$ and $\Delta\beta$. The magnetooptical parameters are the strongest at energies around the absorption edge of the investigated material and vanish at energies far from resonance. The theoretically calculated energy dependency of $\Delta\delta$ and $\Delta\beta$ can be found in Fig. 1 in the main text.

## XRMR Data analysis

The analysis of the collected XRR and asymmetry ratio data was done using ReMagX[3–5]. For fitting the nonmagnetic reflectivity $I$, the recursive Parratt algorithm[6] was used, while the roughness was modelled within a Névot-Croce approximation[7]. The fit of the asymmetry ratio is based on the Zak matrix formalism[8]. As described in Ref.[9,10],


[a)] Electronic mail: dgraulich@physik.uni-bielefeld.de

the structural parameters, i.e. the thicknesses and roughnesses of the different layers in the stacks, are obtained by fitting an additionally taken off-resonant XRR curve (not shown). At a photon energy significantly away from the absorption edge, here 100 eV below, the optical parameters can be taken from literature[11]. Allowing for only slight variations of these obtained structural parameters[5], the averaged resonant XRR curves were fitted by additionally varying the optical parameters.

As stated in the main text, the energy for the XRMR measurements was chosen to minimize the effect of $\Delta\delta$ in accordance with the ab initio calculation. When performing a Kramers-Kronig transformation of the XMCD signal as shown in Fig. S1, it can also experimentally be seen, that the magnetooptic dispersion is close to zero for the energy, which was chosen to be at the maximum of the XMCD signal.

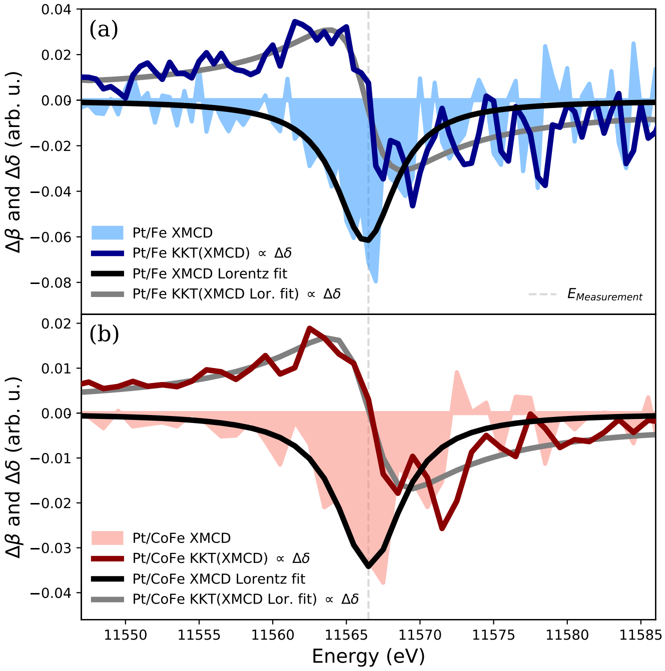


FIG. S1. XMCD signal (filled area) together with the corresponding Kramers-Kronig transformation for (a) the Pt/Fe sample and (b) the $Pt/Co_{33}Fe_{67}$ sample. Additionally shown in black are the Lorentz fits of the XMCD signal and in grey the Kramers-Kronig transformation of that fit. The dashed grey vertical line indicates the energy chosen for the measurements.

For the Pt $L_3$ edge, the energy resolution of the beamline is $\pm 0.5$ eV. Taking this energy window into account, the XRMR experiments were still carried out within the maximum of $\Delta\beta$ and any influence of $\Delta\delta$ is negligible.

## Comparison of XRMR and XMCD Results

To quantitatively compare the spin magnetic moments as obtained from the XRMR analysis to the XMCD sum-rule analysis, we consider the integration of both results. For XRMR, we take the $\Delta\beta$ depth profile from the XRMR fitting, scaled by the ab initio factor to units of $\mu_B$. For the XMCD results, we got a magnetic moment that is the average over the complete Pt layer. Therefore, we take the normalized Pt density depth profiles, taken from the XRMR fits, and scale them o the spin magnetic moment from the sum-rule analysis.

$$A_{\mathrm{XRMR}} = \int_{\mathrm{mag.\ Pt}} \Delta\beta \cdot \text{ab initio conv. factor} \quad ; \quad A_{\mathrm{XMCD}} = \int_{\mathrm{total\ Pt}} \text{normalized Pt density} \cdot \mu_{\mathrm{spin}}^{\mathrm{XMCD}} \tag{S1}$$

The ratios between those areas, $A_{XMCD}/A_{XRMR}$, are 0.96 and 0.94 for Pt/Fe and $Pt/Co_{33}Fe_{67}$, respectively. The scaled magnetic depth profiles can be seen in Fig. S2.

Another possibility is to calculate the scaling factor needed for the $\Delta\beta$ depth profiles to units of $\mu_B$, so that a subsequent integration fulfils $A_{XMCD}$=$A_{XRMR}$. When taking the maximum values from the resulting scaled depth profiles, we get $0.45\pm0.14\,\mu_B$ and $0.63\pm0.22\,\mu_B$ for Pt/Fe and $Pt/Co_{33}Fe_{67}$, respectively. This approach of converting the averaged XMCD moment to the real moment at the interface via the areas $A_{XMCD}$ and $A_{XRMR}$ is slightly

more accurate than just using the total Pt thickness and the effective thickness of the magnetic Pt (FWHM of the Gaussian-like $\Delta\beta$ depth profile) for this conversion as we have done in prior works[10,12].

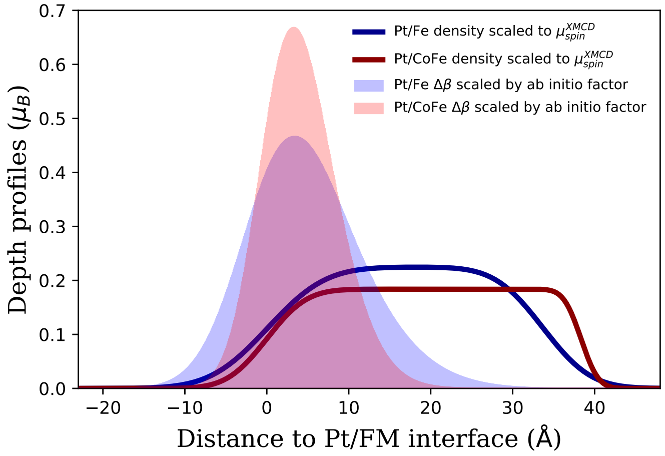


FIG. S2. The magnetic depth profiles from the XRMR and XMCD analysis. The $\Delta\beta$ depth profiles are converted by the ab initio factor into units of $\mu_B$. For the XMCD anlysis, the normalized Pt density depth profile from the XRMR fit is multiplied by the spin magnetic moment $\mu_{\rm spin}^{\rm XMCD}$ obtained from the XMCD sum-rule analysis.

## Determination of Error Bars

For the XRMR measurements, the error bars are determined by varying the XRR and XRMR asymmetry ratio parameters while keeping the increase of the goodness of fit ($\chi^2$ value) below 10 %, a rough hallmark for which the differences between experimental data and fit curve became visible by eye. For all these individual changes, the magnetic moment and FWHM have been calculated and the errors displayed in Tab. I of the main text are upper limits for the observed variations.

The uncertainties in the application of the sum rules and the resulting values stem from the integration of the partly noisy data, especially the XMCD signal, and have been estimated by calculating a maximum error, with each error contribution of the integration taken as ±10%. Due to the large uncertainties in the evaluation of the orbital moments, an upper limit is displayed instead of providing a value with error bars. For both samples, these upper limits of orbital moments are within the order of magnitude of the spin moment error.

## Discussion on the Orbital Moments

In another study[13] a larger orbital moment was found for $Co_xFe_{1-x}$ alloys, which resemble the stoichiometry of our used $Co_{33}Fe_{67}$, compared to pure Fe. However, within our XMCD analysis we found the upper limit for the orbital Pt moment to be larger within the Pt/Fe sample when compared to Pt/$Co_{33}Fe_{67}$. This might be explained by the general uncertainty in the estimation of the orbital moment, which corresponds to the difference in the XMCD signal between $L_3$ and $L_2$ within the sum rule analysis, a value especially prone to the general uncertainties due to the signal-to-noise ratio within the measurements. Another explanation might be the larger interfacial roughness of the Pt/Fe sample, which seems to broaden the spin depth profile obtained within the XRMR analysis. In an XMCD study of thin Pt layers with different thicknesses, a difference in the decay of the orbital and spin moments was observed[14]. While the total moment decays exponentially for thicker Pt layers, the ratio between orbital and spin moment got smaller for increased Pt thickness, suggesting a faster decay of the orbital moment. If the interfacial roughness influences the orbital moment the same way as it seems to do for the spin moment, a broader orbital depth profile within the Pt of the Pt/Fe sample can be assumed. Additionally, the Pt itself is thinner in the Pt/Fe sample as obtained from the XRR fits, see Table I in the main text, and as discussed, the non-magnetic Pt does not contribute to the dichroic signal. These factors together might explain why the Pt/Fe seems to have a substantially larger induced Pt orbital moment, while the inducing orbital moment within the Pt/$Co_{33}Fe_{67}$ should in principle be larger. Further investigations related to the induced Pt orbital moment will be done when signal-to-noise ratio will have been improved significantly.

[1] J. Strempfer, S. Francoual, D. Reuther, D. K. Shukla, A. Skaugen, H. Schulte-Schrepping, T. Kracht, and H. Franz, J. Synchrotron Radiat. **20**, 541 (2013).
[2] P. Bougiatioti, O. Manos, O. Kuschel, M. Tolkiehn, S. Francoual, and T. Kuschel, arXiv:1807.09032 (2018).

[3] S. Macke, A. Radi, J. E. Hamann-Borrero, A. Verna, M. Bluschke, S. Brück, E. Goering, R. Sutarto, F. He, G. Cristiani, M. Wu, E. Benckiser, H.-U. Habermeier, G. Logvenov, N. Gauquelin, G. A. Botton, A. P. Kajdos, S. Stemmer, G. A. Sawatzky, M. W. Haverkort, B. Keimer, and V. Hinkov, Adv. Mater. **26**, 6554 (2014).
[4] S. Macke and E. Goering, J. Phys: Condens. Matter **26**, 363201 (2014).
[5] J. Krieft, D. Graulich, A. Moskaltsova, L. Bouchenoire, S. Francoual, and T. Kuschel, J. Phys. D: Appl. Phys. **53**, 375004 (2020).
[6] L. G. Parratt, Phys. Rev. **95**, 359 (1954).
[7] L. Névot and P. Croce, Rev. Phys. Appl. **15**, 761 (1980).
[8] J. Zak, E. R. Moog, C. Liu, and S. D. Bader, J. Magn. Magn. Mater. **89**, 107 (1990).
[9] C. Klewe, T. Kuschel, J.-M. Schmalhorst, F. Bertram, O. Kuschel, J. Wollschläger, J. Strempfer, M. Meinert, and G. Reiss, Phys. Rev. B **93**, 214440 (2016).
[10] T. Kuschel, C. Klewe, J. M. Schmalhorst, F. Bertram, O. Kuschel, T. Schemme, J. Wollschläger, S. Francoual, J. Strempfer, A. Gupta, M. Meinert, G. Götz, D. Meier, and G. Reiss, Phys. Rev. Lett. **115**, 097401 (2015).
[11] B. L. Henke, E. M. Gullikson, and J. C. Davis, At. Data Nucl. Data Tables **54**, 181 (1993).
[12] S. Geprägs, C. Klewe, S. Meyer, D. Graulich, F. Schade, M. Schneider, S. Francoual, S. P. Collins, K. Ollefs, F. Wilhelm, A. Rogalev, Y. Joly, S. T. B. Goennenwein, M. Opel, T. Kuschel, and R. Gross, Phys. Rev. B, accepted, arXiv:2010.03979 (2020).
[13] M. A. W. Schoen, J. Lucassen, H. T. Nembach, T. J. Silva, B. Koopmans, C. H. Back, and J. M. Shaw, Phys. Rev. B **95**, 134410 (2017).
[14] M. Suzuki, H. Muraoka, Y. Inaba, H. Miyagawa, N. Kawamura, T. Shimatsu, H. Maruyama, N. Ishimatsu, Y. Isohama, and Y. Sonobe, Phys. Rev. B **72**, 054430 (2005).
